# Supplementary material for: Extracting the gamma-ray source-count distribution below the Fermi-LAT detection limit with deep learning
Source: arXiv:2302.01947 source file (2024-05-15)
Supplement: Supplementary file 1 [file appendix_A.tex]

\section{Appendice}
Una appendice
